# Supplementary material for: Distinct Shortest Walk Enumeration for RPQs
Source: arXiv:2312.05505 source file (2024-03-07)
Supplement: Supplementary file 1 [file C-linear-in-automata.tex]

\newappendix{Attaining linear complexity}
\label{appendix:linear in automata}
